# Supplementary material for: Mapping representations in Reinforcement Learning via Semantic Alignment for Zero-Shot Stitching
Source: arXiv:2503.01881 source file (2025-02-26)
Supplement: Supplementary file 1 [file appendix.tex]

\subsection{envs}

For the following experiments, we consider the CarRacing \citep{klimov2016carracing} environment, which simulates driving a car from a 2D top-down perspective around a randomly generated track, focusing on speed while staying on the track. It provides RGB image observations, and uses a discretized action space with five options: steer left, steer right, accelerate, brake, and idle. The agent earns rewards for progress and penalties for going off-track. We modified the environment to enable visual changes (e.g, grass color or camera zoom) and task alterations (e.g., speed limits or different action spaces).
The possible visual variations are: background (grass) colors \textit{green}, \textit{red}, \textit{blue} and \textit{far camera zoom}, while tasks are divided in: \textit{standard} and \textit{slow} car dynamics and different action spaces, such as \textit{scrambled}, which use a different action space and therefore a different output order for the car commands, and \textit{no idle}, which removes the \say{idle} action.
Please refer to \Cref{appendix:atari} for the implementation and tests with another environment.

\paragraph{CleanRL training implementatino}
with default hypermarameters for both absolute and relative representations. \AR{Scrivi hyperparam}

\subsection{maths}

To obtain a transformation \tau_u^v, we rely on the Singular Value Decomposition (SVD) of paired latent samples, as similarly done in prior alignment works (Maiorca et al., 2023; Moschella et al., 2023). Specifically, we collect corresponding datasets \mathbf{X}_u and \mathbf{X}_v by following the same procedure used in R3L [citation]. Let \bar{\mathbf{x}}_u and \bar{\mathbf{x}}_v be the mean embeddings for these two datasets, respectively. Denote the centered versions as:

\widetilde{\mathbf{X}}_u \;=\; \mathbf{X}_u - \bar{\mathbf{x}}_u,
\quad\quad
\widetilde{\mathbf{X}}_v \;=\; \mathbf{X}_v - \bar{\mathbf{x}}_v.

We then compute the SVD of \widetilde{\mathbf{X}}_v^\mathsf{T}\,\widetilde{\mathbf{X}}_u:

\widetilde{\mathbf{X}}_v^\mathsf{T}\,\widetilde{\mathbf{X}}_u
\;=\;
\mathbf{U}\,\boldsymbol{\Sigma}\,\mathbf{V}^\mathsf{T}.

An orthogonal alignment matrix can be obtained by

\mathbf{R} \;=\; \mathbf{V}\,\mathbf{U}^\mathsf{T},

and the translational offset by

\mathbf{b}
\;=\;
\bar{\mathbf{x}}_v \;-\; \mathbf{R}\,\bar{\mathbf{x}}_u.

Hence, the desired transformation \tau_u^v takes the form

\tau_u^v(\mathbf{x})
\;=\;
\mathbf{R}\,\mathbf{x} \;+\; \mathbf{b}.

Intuitively, \mathbf{R} captures rotation and (if desired) reflection, while \mathbf{b} accounts for differences in mean position between the two latent spaces. Once this transform is estimated, any latent embedding from \mathbf{X}_u can be mapped to the space of \mathbf{X}_v, enabling zero-shot stitching of separately trained modules without additional fine-tuning.

---

Standard Scaling

Before estimating the alignment transform \tau_u^v, we apply standard scaling to each latent dimension. Concretely, let \mu and \sigma be the per-dimension mean and standard deviation computed on the anchor set (Section X). We then transform each embedding \mathbf{x} by

\mathbf{x}^\mathrm{scaled}
\;=\;
\frac{\mathbf{x} \;-\; \mu}{\sigma},

making all dimensions zero-mean, unit-variance. Standard scaling helps stabilize the subsequent SVD and prevents any single dimension from dominating the alignment. Once the transform \tau_u^v is found in scaled space, we invert this normalization step at inference time where needed, ensuring consistent dimensions for zero-shot stitching.

-----

Estimating \tau via Least Squares

Recall from Section X that we define an affine transformation

\tau: \mathbf{x} \;\mapsto\; \mathbf{W}\,\mathbf{x} \;+\; \mathbf{b},

where \mathbf{W} is a linear operator and \mathbf{b} a (possibly zero) bias term. In our setting, \tau must map embeddings \mathbf{X}_u \in \mathbb{R}^{m \times d} (from domain u) to \mathbf{X}v \in \mathbb{R}^{m \times d} (from domain v), minimizing

\min{\mathbf{W}, \,\mathbf{b}} \;\bigl\|\mathbf{X}_u\,\mathbf{W} \;+\; \mathbf{1}\,\mathbf{b}^{\mathsf{T}}
\;-\;
\mathbf{X}_v
\bigr\|_F^2.

This yields a matrix \mathbf{W}_{\mathrm{est}} that aligns \mathbf{X}_u to \mathbf{X}_v.
	•	If only a linear mapping is desired, we set \tau(\mathbf{x}) = \mathbf{W}_{\mathrm{est}} \mathbf{x}, ignoring bias.
	•	For a full affine transform, we can either include a column of ones in \mathbf{X}_u to solve for \mathbf{b} directly, or do a mean-centering trick to recover \mathbf{b} from the offset in means.

Once \mathbf{W} and (optionally) \mathbf{b} are computed, we apply

\tau(\mathbf{x})
\;=\;
\mathbf{W}_{\mathrm{est}}\mathbf{x}
\;+\;
\mathbf{b}

to any new latent \mathbf{x} in domain u, effectively translating it to the space of domain v.
